# Supplementary material for: Quantum scattering model of energy transfer in photosynthetic complexes
Source: arXiv:1201.1740 source file (2012-01-09)
Supplement: Supplementary file 1 [file suppl.pdf]

# Supplementary material for 'Quantum scattering model of energy transfer in photosynthetic complexes'

Bao-quan Ai[1] and Shi-Liang Zhu[1,2]
[1]*Laboratory of Quantum Information Technology and SPTE, South China Normal University, Guangzhou, China*
[2] *Center for Quantum Information, IIIS, Tsinghua University*

In this supplementary material, we review some basic results of the quantum scattering model developed in the condensed matter physics[1–3]. Furthermore, we provide several examples to demonstrate our basic ideas on the optimal quantum transport.

## A. INTRODUCTION OF QUANTUM SCATTERING MODEL

In this section, we provide the transfer matrices for the scatterer, an array of the scatterers, the junctions $S$ and $G$ used in the paper.

(a) *Transfer Matrix for a scatterer and an array of the scatterers.* We consider a particle pass through a barrier shown in Fig. 1. The wave function could be written as

$$\psi(x) = \begin{cases} C_L e^{ikx} + D_L e^{-ikx}, & \text{as } x < x_1; \\ C_R e^{ikx} + D_R e^{-ikx}, & \text{as } x > x_2, \end{cases} \quad (1)$$

where $k$ is the wave number, $C_{L(R)}$ and $D_{L(R)}$ are the amplitudes of the wave function at the left (right) of the scatterer.

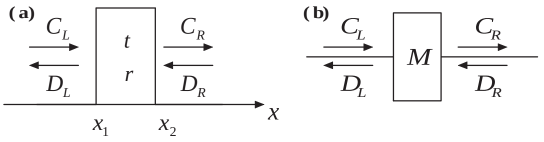


FIG. 1: (a) Schematic representation of the potential $V(x)$. (b) The symbol of a scatterer. The transfer matrix relates the amplitudes $C_L$, $D_L$ to $C_R$, $D_R$.

Instead of a potential $V(x)$, we describe the elastic scattering in pathway with the help of the transfer matrix. From Fig. 1, we can find that the outgoing waves with amplitudes ($D_L$, $C_R$) are related to the incoming waves ($C_L$,$D_R$)

$$D_L = rC_L + tD_R \quad (2)$$
$$C_R = tC_L + rD_R, \quad (3)$$

where $t$ and $r$ are the transmission and reflection amplitudes, respectively. Equations (2) and (3) can be rewritten as the matrix form

$$\begin{pmatrix} D_L \\ C_R \end{pmatrix} = \Upsilon \begin{pmatrix} C_L \\ D_R \end{pmatrix}, \Upsilon = \begin{pmatrix} r & t \\ t & r \end{pmatrix}. \quad (4)$$

$\Upsilon$ is the scattering matrix of the scatterer. Current conservation implies that $\Upsilon$ is unitary, $\Upsilon^\dagger\Upsilon = \Upsilon\Upsilon^\dagger = 1$. Therefore, we can obtain $rt^* + tr^* = 0$. The asterisk denotes complex conjugation. By rewriting Eq. (4), the amplitudes $C_L$, $D_L$ of the wave function on the left of the scatterer can be related to the amplitudes $C_R$, $D_R$ on the right by the following matrix equation,

$$\begin{pmatrix} C_R \\ D_R \end{pmatrix} = M \begin{pmatrix} C_L \\ D_L \end{pmatrix}, \quad (5)$$

where $M$ is the transfer matrix for the scatterer and can be written as

$$M = \begin{pmatrix} 1/t^* & -r^*/t^* \\ -r/t & 1/t \end{pmatrix}, \quad (6)$$

where $t{=}T^{\frac{1}{2}}e^{i\varphi}$, $r{=}{-}iR^{\frac{1}{2}}e^{i\varphi}$, $T$ is the transmission probability for the scatterer, $R{=}1-T$ is its reflection probability. $\varphi$ is the phase change in the transmitted wave and we set $\varphi = 0$ just for simplicity in this paper.

Similarly, we can also obtain the transfer matrix $U_l$ for the ideal path,

$$U_l = \begin{pmatrix} e^{-ikl} & 0 \\ 0 & e^{ikl} \end{pmatrix}, \quad (7)$$

where $l$ is the length of the ideal path.

Based on the transfer matrixes $M$ and $U_l$, we can obtain the transfer matrix $L$ for an array of the scatterers shown in Fig. 2. The transfer matrix $L$ relates the amplitudes $C_L$ and $D_L$ to $C_R$ and $D_R$ through the relation given by

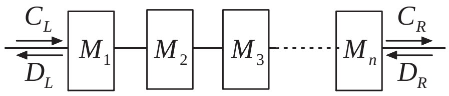


FIG. 2: Schematic picture for an array of the scatterers.

$$\begin{pmatrix} C_R \\ D_R \end{pmatrix} = L \begin{pmatrix} C_L \\ D_R \end{pmatrix}, \quad (8)$$

where $L = M_n U_{l_{n-1}} M_{n-1} ... M_2 U_{l_1} M_1$.

(b) *Scattering matrix for S Junction.* As the junction shown in Fig. 3 (a), the three outgoing waves with amplitude $\overrightarrow{\alpha_o}(I_o, x_o, y_o)$ are related by a $S$ matrix to the

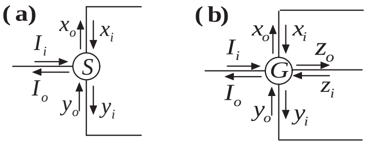


FIG. 3: Schematic picture for junctions $S$ and $G$. (a) $S$ junction; (b) $G$ junction. The symbols near the arrows denote the corresponding amplitudes of the incoming and outgoing wave function.

three incoming waves $\overrightarrow{\alpha_i}(I_i, x_i, y_i)$, $\overrightarrow{\alpha_o} = S\overrightarrow{\alpha_i}$. A simple choice that $S$ is real and symmetric with respect to the two branches is given by

$$S = \begin{pmatrix} a & b & b \\ b & c & d \\ b & d & c \end{pmatrix}, \tag{9}$$

where each diagonal element, $S_{i,i}$, denotes the reflection amplitude of the $i$th branch, and off-diagonal elements, $S_{i,j}(i \neq j)$ are the transmission amplitudes from branch $i$ to $j$. Probability conservation requires $S^\dagger S = SS^\dagger = 1$ and the coefficients $a$, $b$, $c$, and $d$ then satisfy the following equations,

$$\begin{aligned} a^2 + 2b^2 &= 1, & (10) \\ b^2 + c^2 + d^2 &= 1, & (11) \\ ab + bc + bd &= 0, & (12) \\ b^2 + 2cb &= 0. & (13) \end{aligned}$$

When the junction is completely transparent for incoming $I$ which requires $a = 0$. From Eqs. (10-13) we can obtain $b = \frac{1}{\sqrt{2}}$, $c = \frac{1}{2}$ and $d = -\frac{1}{2}$ and thus

$$S = \begin{pmatrix} 0 & \frac{1}{\sqrt{2}} & \frac{1}{\sqrt{2}} \\ \frac{1}{\sqrt{2}} & \frac{1}{2} & -\frac{1}{2} \\ \frac{1}{\sqrt{2}} & -\frac{1}{2} & \frac{1}{2} \end{pmatrix}. \tag{14}$$

(c)*Scattering matrix for G Junction* . For junction $G$ shown in Fig. 3(b), the four outgoing waves with amplitude $\overrightarrow{\beta_o}(I_o, x_o, y_o, z_o)$ are related by a $G$ matrix to the four incoming waves $\overrightarrow{\beta_i}(I_i, x_i, y_i, z_i)$, $\overrightarrow{\beta_o} = G\overrightarrow{\beta_i}$. We assume that the junction $G$ contains one input branch $I$ and three identical output branches $x$, $y$, and $z$. Therefore, the real matrix $G$ has four independent parameters and can be written as

$$G = \begin{pmatrix} a & b & b & b \\ b & c & d & d \\ b & d & c & d \\ b & d & d & c \end{pmatrix}, \tag{15}$$

where the diagonal element denotes the reflection amplitude and the off-diagonal elements are the transmission amplitudes. The matrix $G$ is unitary, $G^\dagger G = GG^\dagger = 1$ and the coefficients $a$, $b$, $c$, and $d$ satisfy the following relations

$$\begin{aligned} a^2 + 3b^2 &= 1, & (16) \\ b^2 + c^2 + 2d^2 &= 1, & (17) \\ ab + bc + 2bd &= 0, & (18) \\ b^2 + d^2 + 2cd &= 0. & (19) \end{aligned}$$

Similar to the junction $S$, we also consider the case where the junction is completely transparent for incoming $I$ which requires $a = 0$. From Eqs. (16-19). one can find $b = \frac{1}{\sqrt{3}}$, $c = \frac{2}{3}$, $d = -\frac{1}{3}$. Therefore, the matrix $G$ can be written as

$$G = \begin{pmatrix} 0 & \frac{1}{\sqrt{3}} & \frac{1}{\sqrt{3}} & \frac{1}{\sqrt{3}} \\ \frac{1}{\sqrt{3}} & \frac{2}{3} & -\frac{1}{3} & -\frac{1}{3} \\ \frac{1}{\sqrt{3}} & -\frac{1}{3} & \frac{2}{3} & -\frac{1}{3} \\ \frac{1}{\sqrt{3}} & -\frac{1}{3} & -\frac{1}{3} & \frac{2}{3} \end{pmatrix}. \tag{20}$$

## B. SEVERAL SIMPLE EXAMPLES

To well understand the scattering model and the main ideas in the paper, we here present the main results of quantum and classical transports for three simple configurations. We focus on finding whether the transport involved quantum behaviors is more efficient than that involved classical behaviors and whether the number of the pathways affects the transport. For simplicity, We assume that all scatterers have the same transmission probability $T$.

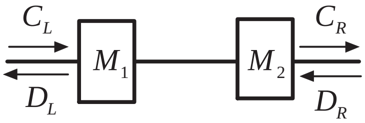


FIG. 4: Schematic picture for the single pathway with two scatterers.

(a)*Single pathway.* Firstly, we study the particle transport through the single pathway with two scatterers shown in Fig. 4. With help of the transfer matrixes of the scatterers, we can obtain the relation of the amplitudes $C_L$, $D_L$ to $C_R$, $D_R$,

$$\begin{pmatrix} C_R \\ D_R \end{pmatrix} = L \begin{pmatrix} C_L \\ D_L \end{pmatrix}, \tag{21}$$

where $L = M_2 U_{l_1} M_1$ with $l_1$ being the distance between the two scatterers. By setting $C_L = 1$ and $D_R = 0$, we obtain the total transmission probability $T_{total} = |C_R|^2$ as

$$T_{total} = \frac{T^2}{T^2 + 4(1-T)\cos^2\phi_1}, \tag{22}$$

where $\phi_1 = kl_1$. When $\phi_1 = \frac{n}{2}\pi$ ($n$ is odd number), $T_{total}$=1, the resonant tunneling will happen.

After considering the multi-reflection between the s-catterers $M_1$ and $M_2$, we may obtain the classical transmission probability as

$$T_C = T^2(1 + R^2 + R^4 + R^6 + ...). \tag{23}$$

Here the first term represents the probability of the particle directly pass through the two scatterers, the second term represents the transmission after reflected one time by the scatterer $M_2$ and so on. $T_C$ is the sum of a geometric series with the common ratio $R^2$. So we can obtain $T_C = \frac{T}{2-T}$.

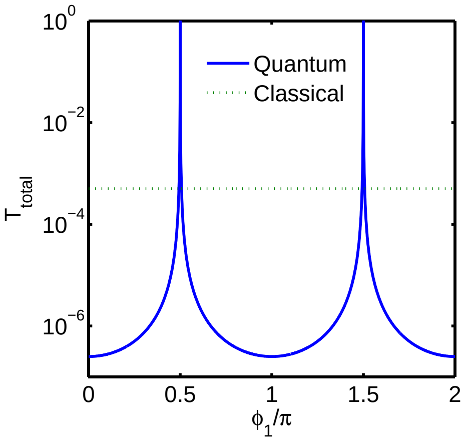


FIG. 5: (Color online)The total transmission probability $T_{total}$ as a function of the path phases $\phi_1$ for both quantum and classical cases at $T = 0.001$.

Figure 5 shows the total transmission probability as a function of the path phase for both quantum and classical cases at strong scattering limit $T = 0.001$. For classical case, $T_C = 5 \times 10^{-4}$, it is impossible for the particle to pass through the system at strong scattering limit. However, for quantum case, there exists two resonant peaks at which the total transmission probability takes its maximal value $T_{total} = 1$. Therefore, the transport involved optimal quantum coherence is more efficient than that involved the classical behaviors alone.

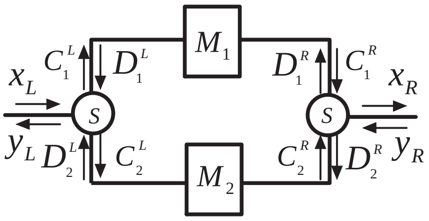


FIG. 6: Schematic picture for two pathways with two $S$ junctions.

(b)*Double pathways.* Two pathways form a ring and connected to two leads through two $S$ junctions shown in Fig. 5 For each pathway, the transfer matrix $L_j$ ($j = 1, 2$) relates the amplitudes $C_j^L$, $D_j^L$ to the amplitudes $C_j^R$, $D_j^R$

$$\begin{pmatrix} C_j^R \\ D_j^R \end{pmatrix} = L_j \begin{pmatrix} C_j^L \\ D_j^L \end{pmatrix}, \tag{24}$$

where $L_j = U_{l_j} M_j U_{l_j}$ and $l_j$ is the distance between the junction $S$ and the $j$th scatterer.

The amplitudes of the three outgoing waves are related to the amplitudes of the three incoming waves through the $S$ matrix given by

$$\begin{pmatrix} y_L \\ C_1^L \\ C_2^L \end{pmatrix} = S \begin{pmatrix} x_L \\ D_1^L \\ D_2^L \end{pmatrix}, \quad \begin{pmatrix} x_R \\ D_1^R \\ D_2^R \end{pmatrix} = S \begin{pmatrix} y_R \\ C_1^L \\ C_2^L \end{pmatrix}. \tag{25}$$

From Eqs. (24) and (25), we can find the total transmission probability of the double pathways $T_{total} = |x_R|^2$ at $x_L = 1$ and $y_R = 0$,

$$T_{total} = \frac{H^2}{P^2 + Q^2}, \tag{26}$$

where $H = \sqrt{T}[2\sqrt{R} + \sin 2\phi_1 + \sin 2\phi_2]$, $P = 2\sin^2(\phi_1 + \phi_2) - \sin^2(\phi_1 - \phi_2) + \sqrt{R}(\sin 2\phi_1 + \sin 2\phi_2)$, $Q = \sin 2(\phi_1 + \phi_2) + \sqrt{R}(\cos 2\phi_1 + \cos 2\phi_2)$, $\phi_j = kl_j$.

When $\phi_1 = \phi_2$, $T_{total} = T$. When $\phi_1 + \phi_2 = \frac{\pi}{2}$, $T_{total} = 0$ for $\phi_1 = \frac{1}{2}\arcsin(-\sqrt{R})$ and $T_{total} = 1$ for $\phi_1 = \frac{1}{2}\arcsin(\sqrt{T} - \sqrt{R})$.

For classical case, it is very difficult to find the total classical transmission probability $T_C$. However, we can obtain the minimal reflected probability $R_{min}$ from the left of the system

$$R_{min} = \frac{1}{2}R + \frac{1}{4}R^2 + \frac{1}{8}R^3 + .... = \frac{R}{2 - R}. \tag{27}$$

Here the first term represents the reflected probability after directly reflected one time by the scatterers $M_1$ and $M_2$, the second terms represents the reflected probability after directly reflected two times by the scatterers $M_1$ and $M_2$ and so on. The upper bound of total classical transmission probability is $1 - R_{min} = \frac{2T}{1+T}$, thus $T_C < \frac{2T}{1+T}$.

Figure 7 shows the total transmission probability as functions of the path phases at $T = 0.05$. For classical case, $T_C < 0.095$, the particle passes through the system with very small probability. However, for quantum case, there are eight resonant regions where the particle can pass through the system without any loss. Compared with the single pathway, the resonant regions for two pathways become larger and it is easier for the particle to pass through the system.

(c) *Three pathways.* Three pathways form two rings and connected to two leads through two $G$ junctions shown in Fig. 6. The left amplitudes $C_j^L$, $D_j^L$ of the

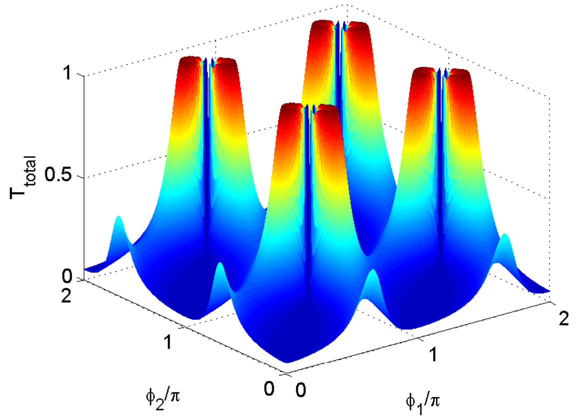


FIG. 7: (Color online)The total transmission probability $T_{total}$ as functions of the path phases $\phi_1$ and $\phi_2$ at $T = 0.05$.

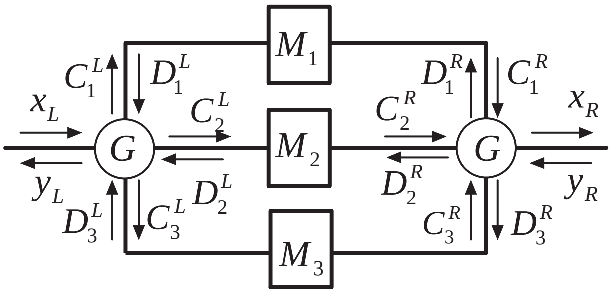

FIG. 8: Schematic picture for three pathways with two $G$ junctions.

scatterer are related to the right amplitudes $C_j^R$, $D_j^R$ by the effective transfer matrix $L_j$ $(j = 1, 2, 3)$,

$$\begin{pmatrix} C_j^R \\ D_j^R \end{pmatrix} = L_j \begin{pmatrix} C_j^L \\ D_j^L \end{pmatrix}, \tag{28}$$

where $L_j = U_{l_j} M_j U_{l_j}$ and $l_j$ is the distance between the junction $G$ and the $j$th scatterer.

The amplitudes of the four outgoing waves are related by a $G$ matrix to the amplitudes of the four incoming waves

$$\begin{pmatrix} y_L \\ C_1^L \\ C_2^L \\ C_3^L \end{pmatrix} = G \begin{pmatrix} x_L \\ D_1^L \\ D_2^L \\ D_3^L \end{pmatrix}, \quad \begin{pmatrix} x_R \\ D_1^R \\ D_2^R \\ D_3^R \end{pmatrix} = G \begin{pmatrix} y_R \\ C_1^R \\ C_2^R \\ C_3^R \end{pmatrix}, \tag{29}$$

From Eqs. (28) and (29), we can find the total transmission probability of the three pathways $T_{total} = |x_R|^2$ at $x_L = 1$ and $y_R = 0$,

$$T_{total} = \frac{H^2}{P^2 + Q^2}, \tag{30}$$

where $H = 3\sqrt{T}[3R + 2\sqrt{R}(\sin 2\phi_1 + \sin 2\phi_2 + \sin 2\phi_3) + \sin 2\phi_1 \sin 2\phi_2 + \sin 2\phi_1 \sin 2\phi_3 + \sin 2\phi_2 \sin 2\phi_3]$, $P = 3(\cos 2\phi_1 \sin 2\phi_2 \sin 2\phi_3 + \cos 2\phi_2 \sin 2\phi_1 \sin 2\phi_3 + \cos 2\phi_3 \sin 2\phi_1 \sin 2\phi_3) + 3\sqrt{R}[\sin 2(\phi_1 + \phi_2) + \sin 2(\phi_1 + \phi_3) + \sin 2(\phi_2 + \phi_3)] + 3R(\cos 2\phi_1 + \cos 2\phi_2 + \cos 2\phi_3)$, $Q = (3R + 1)(\sin 2\phi_1 + \sin 2\phi_2 + \sin 2\phi_3) + [2\cos 2(\phi_1 - \phi_2) + 2\cos 2(\phi_1 - \phi_3) + 2\cos(\phi_2 - \phi_3) - 3\cos 2(\phi_1 + \phi_3) - 3\cos 2(\phi_2 + \phi_3) - 3\cos 2(\phi_1 + \phi_2) + 3]\sqrt{R} - \cos 2\phi_1 \cos 2\phi_2 \sin 2\phi_3 - \cos 2\phi_1 \cos 2\phi_3 \sin 2\phi_2 - \cos 2\phi_2 \cos 2\phi_3 \sin 2\phi_1 + 6 \sin 2\phi_1 \sin 2\phi_2 \sin 2\phi_3$, $\phi_j = kl_j$.

When $\phi_1 = \phi_2 = \phi_3$, $T_{total} = T$. When $\phi_2 = \phi_3$ and $\phi_1 + \phi_2 = \frac{\pi}{2}$, $T_{total} = 0$ for $\phi_1 = \frac{1}{2}\arcsin(-\sqrt{R})$ and $T_{total} = 1$ for $\phi_1 = \frac{1}{2}\arcsin((-9\sqrt{R} + \sqrt{64 - 63R})/8)$.

Similar to the double pathways, the minimal reflected probability $R_{min}$ from the left of the system

$$R_{min} = \frac{1}{3}R + \frac{2}{9}R^2 + \frac{4}{27}R^3 + .... = \frac{R}{3 - 2R}. \tag{31}$$

The upper bound of total classical transmission probability is $1 - R_{min} = \frac{3T}{1+2T}$, thus $T_C < \frac{3T}{1+2T}$.

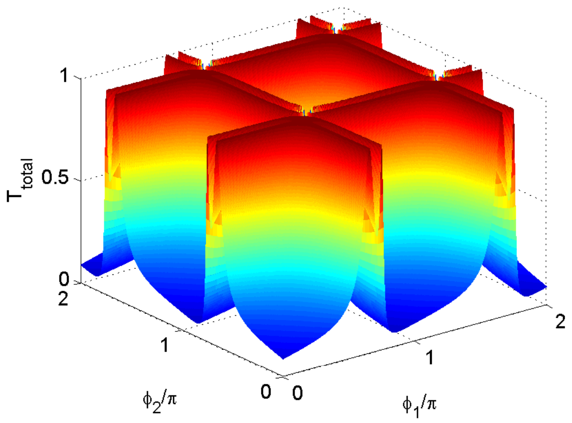


FIG. 9: (Color online)The total transmission probability $T_{total}$ as functions of the path phases $\phi_1$ and $\phi_2$ for $T = 0.05$ and $\phi_3 = \frac{1}{2}\arcsin((-9\sqrt{R} + \sqrt{64 - 63R})/8)$.

Figure 9 shows the relation between the total transmission probability and the path phases at $T = 0.05$. For classical case, $T_C < 0.136$, the efficiency of the transport is very low. Similar to the double pathways, there exist resonant regions for quantum case. Moreover, the resonant regions are larger than that for single, and double pathways. The resonant structures for one, two, and three pathways are shown in Fig. (10) at $T = 0.05$. The resonant regions become larger when the number of the pathways is increased.

From the above discussion on the transmission for different number of pathways, we may obtain the following conclusion: (i) the transport involved optimal quantum coherence is more efficient than that involved the classical behavior alone; (ii) the resonant region becomes larger when the number of the pathways is increased. Therefore, multiple pathways can improve the efficiency of the transfer; (iii) the optimal path phases are critical

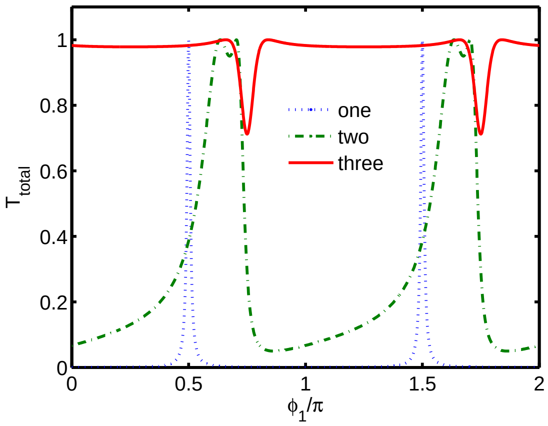


FIG. 10: (Color online)The resonant structures for one, two, and three pathways at $T = 0.05$. (a) One pathway: Eq. (22); (b) two pathways: Eq. (26) at $\phi_2 = \frac{1}{2}\arcsin(\sqrt{T} - \sqrt{R})$; (c)three pathways: Eq.(30) for $\phi_2 = \frac{\pi}{2} - \phi_1$ and $\phi_3 = \frac{1}{2}\arcsin((-9\sqrt{R} + \sqrt{64 - 63R})/8)$.

for the almost perfect efficiency. Therefore, the optimal space distribution of the scatterers, multiple pathways, and quantum behaviors are combined together to ensure high efficiency of the transport.

[1] P. W. Anderson, D. J. Thouless, E. Abrahams, and D. S. Fisher, Phys. Rev. B **22**, 3519 (1980).

[2] M. Buttiker, Y. Imry, and M. Ya. Azbel, Phys. Rev. A **30**, 1982 (1984); Y. Gefen, Y. Imry, and M. Ya. Azbel, Phys. Rev. Lett. **52**, 129 (1984).

[3] S. L. Zhu, and Z. D. Wang, Phys. Rev. Lett. **85**, 1076 (2000); Phys. Rev. B **61**, 1142 (2000).
